# Supplementary material for: Towards a Holistic and Automated Evaluation Framework for Multi-Level Comprehension of LLMs in Book-Length Contexts
Source: arXiv:2508.19578 source file (2025-08-27)
Supplement: Supplementary file 1 [file levels.tex]

% Define colors
\definecolor{good}{RGB}{0,180,0}    % 绿色
\definecolor{bad}{RGB}{255,0,0}     % 红色

\begin{table*}[]
\centering
\resizebox{\textwidth}{!}{%
\begin{tabular}{cccccccccccccc}
\hline
 &  & \multicolumn{3}{c}{Root Completeness} & \multicolumn{3}{c}{Branch Completeness} & \multicolumn{3}{c}{Leaf Completeness} & \multicolumn{3}{c}{MDR} \\ \cline{3-14} 
 &  & Ana. & Nar. & Avg. & Ana. & Nar. & Avg. & Ana. & Nar. & Avg. & Ana. & Nar. & Avg. \\ \hline
\multirow{3}{*}{strong} & GPT-4o & \cellcolor{good!60}0.87 & \cellcolor{good!60}0.90 & \cellcolor{good!60}0.88 & \cellcolor{good!60}0.52 & \cellcolor{good!60}0.56 & \cellcolor{good!60}0.54 & \cellcolor{good!30}0.18 & \cellcolor{good!60}0.29 & \cellcolor{good!60}0.23 & \cellcolor{good!60}0.51 & \cellcolor{good!60}0.44 & \cellcolor{good!60}0.47 \\
 & Claude-3.5-Sonnet & \cellcolor{bad!28}0.82 & \cellcolor{bad!7}0.86 & \cellcolor{bad!30}0.84 & \cellcolor{good!60}0.52 & \cellcolor{good!60}0.56 & \cellcolor{good!60}0.54 & \cellcolor{good!60}0.20 & \cellcolor{good!60}0.30 & \cellcolor{good!60}0.25 & \cellcolor{good!45}0.50 & \cellcolor{good!60}0.44 & \cellcolor{good!52}0.47 \\
 & Llama-3.1-405B-Instruct & \cellcolor{good!60}0.87 & \cellcolor{good!60}0.90 & \cellcolor{good!60}0.88 & \cellcolor{bad!11}0.49 & \cellcolor{good!30}0.54 & \cellcolor{good!15}0.52 & \cellcolor{bad!30}0.15 & \cellcolor{bad!45}0.24 & \cellcolor{bad!35}0.20 & \cellcolor{good!15}0.49 & \cellcolor{good!15}0.41 & \cellcolor{good!15}0.45 \\ \hline
\multirow{3}{*}{weak} & GPT-4o-mini & \cellcolor{good!34}0.86 & \cellcolor{good!24}0.88 & \cellcolor{good!30}0.87 & \cellcolor{good!9}0.50 & \cellcolor{bad!45}0.48 & \cellcolor{bad!30}0.49 & \cellcolor{bad!15}0.16 & \cellcolor{bad!60}0.21 & \cellcolor{bad!45}0.18 & \cellcolor{bad!30}0.48 & \cellcolor{bad!60}0.39 & \cellcolor{bad!45}0.43 \\
 & Claude-3.5-Haiku & \cellcolor{bad!60}0.79 & \cellcolor{bad!60}0.81 & \cellcolor{bad!60}0.80 & \cellcolor{bad!11}0.49 & \cellcolor{good!15}0.53 & \cellcolor{good!0}0.51 & \cellcolor{good!30}0.18 & \cellcolor{good!15}0.26 & \cellcolor{good!30}0.22 & \cellcolor{bad!45}0.47 & \cellcolor{bad!30}0.40 & \cellcolor{bad!30}0.44 \\
 & Llama-3.1-8B-Instruct & \cellcolor{good!60}0.87 & \cellcolor{bad!18}0.85 & \cellcolor{good!20}0.86 & \cellcolor{bad!60}0.46 & \cellcolor{bad!60}0.46 & \cellcolor{bad!60}0.46 & \cellcolor{bad!60}0.13 & \cellcolor{bad!60}0.19 & \cellcolor{bad!60}0.16 & \cellcolor{bad!60}0.46 & \cellcolor{bad!60}0.36 & \cellcolor{bad!60}0.41 \\ \hline
 & Average Strong & 0.85 & 0.89 & 0.87 & 0.51 & 0.56 & 0.53 & 0.18 & 0.27 & 0.23 & 0.50 & 0.43 & 0.46 \\
 & Average Weak & 0.84 & 0.85 & 0.84 & 0.49 & 0.49 & 0.49 & 0.15 & 0.22 & 0.19 & 0.47 & 0.38 & 0.43 \\
& Strong-weak Gap & 0.01 & 0.04 & 0.03 & 0.02 & 0.07 & 0.04 & 0.03 & 0.05 & 0.04 & 0.03 & 0.05 & 0.03 \\
 & Avg Total & 0.85 & 0.87 & 0.86 & 0.50 & 0.52 & 0.51 & 0.17 & 0.25 & 0.21 & 0.48 & 0.41 & 0.45 \\ \hline
\end{tabular}%
}
\caption{Breakdown of the fine-grained completeness evaluation result based on key-fact tree across two summarization perspectives.
Ana. refers to analytical perspective; Nar. refers to narrative perspective. MDR: Mid-degradation Rate.}
\label{tab:fullresult_tree}
\end{table*}
