# Supplementary material for: Towards a Holistic and Automated Evaluation Framework for Multi-Level Comprehension of LLMs in Book-Length Contexts
Source: arXiv:2508.19578 source file (2025-08-27)
Supplement: Supplementary file 2 [file table_for_figure3.tex]

\begin{table*}[t]
\centering
\scriptsize
\resizebox{\textwidth}{!}{
\begin{tabular}{ll rrrr rrrr rrrr rrrr rrrr rrrr}
\toprule
Perspective & Model & \multicolumn{4}{c}{0-20} & \multicolumn{4}{c}{20-40} & \multicolumn{4}{c}{40-60} & \multicolumn{4}{c}{60-80} & \multicolumn{4}{c}{80-100} & \multicolumn{4}{c}{avg} \\
\midrule
 &  & Root & Branch & Leaf & Whole & Root & Branch & Leaf & Whole & Root & Branch & Leaf & Whole & Root & Branch & Leaf & Whole & Root & Branch & Leaf & Whole & Root & Branch & Leaf & Whole \\
\cmidrule(lr){3-6} \cmidrule(lr){7-10} \cmidrule(lr){11-14} \cmidrule(lr){15-18} \cmidrule(lr){19-22} \cmidrule(lr){23-26}
\multirow{6}{*}{Analytical}
    &gpt4o & 0.865 & 0.534 & 0.178 & 0.354 & 0.854 & 0.497 & 0.158 & 0.334 & 0.856 & 0.529 & 0.166 & 0.338 & 0.883 & 0.490 & 0.179 & 0.345 & 0.890 & 0.534 & 0.201 & 0.373 & 0.870 & 0.517 & 0.176 & 0.349 \\

    &gpt4o-mini& 0.865 & 0.526 & 0.170 & 0.349 & 0.865 & 0.499 & 0.144 & 0.326 & 0.854 & 0.506 & 0.157 & 0.325 & 0.896 & 0.514 & 0.156 & 0.340 & 0.836 & 0.469 & 0.161 & 0.323 & 0.863 & 0.503 & 0.158 & 0.333 \\
    &claude-3.5-sonnet& 0.824 & 0.529 & 0.192 & 0.358 & 0.835 & 0.532 & 0.171 & 0.349 & 0.802 & 0.517 & 0.171 & 0.334 & 0.824 & 0.508 & 0.194 & 0.354 & 0.809 & 0.540 & 0.265 & 0.405 & 0.819 & 0.525 & 0.198 & 0.360 \\
    &claude-3.5-haiku & 0.800 & 0.504 & 0.173 & 0.337 & 0.802 & 0.468 & 0.142 & 0.308 & 0.764 & 0.499 & 0.170 & 0.321 & 0.798 & 0.453 & 0.162 & 0.314 & 0.783 & 0.534 & 0.229 & 0.377 & 0.789 & 0.492 & 0.175 & 0.331 \\
    &llama-3.1-405b-instruct & 0.877 & 0.512 & 0.148 & 0.332 & 0.880 & 0.482 & 0.137 & 0.318 & 0.844 & 0.509 & 0.149 & 0.321 & 0.860 & 0.451 & 0.151 & 0.314 & 0.874 & 0.508 & 0.183 & 0.352 & 0.867 & 0.492 & 0.153 & 0.327 \\
    &llama-3.1-8b-instruct & 0.883 & 0.468 & 0.123 & 0.305 & 0.860 & 0.433 & 0.113 & 0.287 & 0.840 & 0.485 & 0.116 & 0.292 & 0.902 & 0.465 & 0.153 & 0.325 & 0.847 & 0.474 & 0.146 & 0.316 & 0.866 & 0.465 & 0.130 & 0.305 \\
\midrule
\multirow{6}{*}{Narrative}
    & gpt4o & 0.909 & 0.583 & 0.286 & 0.452 & 0.858 & 0.555 & 0.265 & 0.425 & 0.929 & 0.537 & 0.269 & 0.432 & 0.887 & 0.509 & 0.261 & 0.417 & 0.928 & 0.637 & 0.343 & 0.503 & 0.902 & 0.564 & 0.285 & 0.446 \\
    &gpt4o-mini & 0.892 & 0.512 & 0.227 & 0.398 & 0.854 & 0.469 & 0.205 & 0.363 & 0.902 & 0.451 & 0.187 & 0.355 & 0.873 & 0.462 & 0.201 & 0.369 & 0.864 & 0.522 & 0.214 & 0.389 & 0.877 & 0.483 & 0.207 & 0.375 \\
    &claude-3.5-sonnet & 0.843 & 0.570 & 0.284 & 0.439 & 0.840 & 0.542 & 0.283 & 0.431 & 0.903 & 0.547 & 0.271 & 0.436 & 0.839 & 0.506 & 0.253 & 0.405 & 0.886 & 0.639 & 0.383 & 0.525 & 0.862 & 0.561 & 0.295 & 0.447 \\
    &claude-3.5-haiku & 0.788 & 0.513 & 0.257 & 0.394 & 0.774 & 0.515 & 0.233 & 0.383 & 0.869 & 0.492 & 0.256 & 0.404 & 0.790 & 0.469 & 0.214 & 0.368 & 0.862 & 0.640 & 0.335 & 0.496 & 0.817 & 0.526 & 0.259 & 0.409 \\
    &llama-3.1-405b-instruct & 0.878 & 0.548 & 0.226 & 0.403 & 0.873 & 0.521 & 0.195 & 0.377 & 0.952 & 0.512 & 0.227 & 0.405 & 0.888 & 0.522 & 0.246 & 0.414 & 0.904 & 0.615 & 0.318 & 0.483 & 0.899 & 0.543 & 0.243 & 0.416 \\
    &llama-3.1-8b-instruct & 0.863 & 0.433 & 0.153 & 0.321 & 0.796 & 0.434 & 0.157 & 0.319 & 0.910 & 0.437 & 0.169 & 0.342 & 0.825 & 0.426 & 0.200 & 0.350 & 0.896 & 0.563 & 0.273 & 0.442 & 0.858 & 0.458 & 0.190 & 0.355 \\
\bottomrule
\end{tabular}
}
\caption{Recall performance across different levels and positions and perspectives.}
\label{tab:recall_total}
\end{table*}
