# Supplementary material for: Towards a Holistic and Automated Evaluation Framework for Multi-Level Comprehension of LLMs in Book-Length Contexts
Source: arXiv:2508.19578 source file (2025-08-27)
Supplement: Supplementary file 3 [file 999-appendix_old.tex]

\newpage
\section{Dataset statistics}\label{appendix: dataset_statistics}

% \input{figures/appendix/data_table/dimensions}
% \input{figures/appendix/data_table/levels}

\begin{table*}[h!]
\centering
\scriptsize
\setlength{\tabcolsep}{2pt} % Reduced column spacing
\renewcommand{\arraystretch}{1.1}
\resizebox{\textwidth}{!}{%
\begin{tabular}{cccccccccccccc}
\toprule
Name & Author & Genre & Token Count & Publication Date &  \# Chunks*  & \multicolumn{4}{c}{Analytical} & \multicolumn{4}{c}{Narrative} \\
\cmidrule(lr){7-10}
\cmidrule(lr){11-14}
 & & & & & & Root & Branch & Leaf & Total & Root & Branch & Leaf & Total \\
\midrule
Wyoming Burn & Jerry Fedora & Mystery & 74,392 & Jan 2, 2025 & 19 & 56 & 141 & 270 & 467 & 65 & 164 & 302 & 531 \\
No Place Left to Hide & Megan Lally & Thriller & 85,616 & Jan 7, 2025 & 22 & 58 & 169 & 365 & 592 & 68 & 182 & 351 & 601 \\
Lady's Steed & Eve Langlais & Romance, Fantasy & 89,884 & Dec 24, 2024 & 23 & 61 & 181 & 384 & 626 & 69 & 207 & 382 & 658 \\
The Assassin’s Guide to Babysitting & Natalie C. Parker & Young Adult & 93,337 & Jan 7, 2025 & 24 & 77 & 202 & 387 & 666 & 82 & 225 & 407 & 714 \\
A Conventional Boy: A Laundry Files Novel & Charles Stross & Fantasy, Horror & 96,274 & Jan 7, 2025 & 24 & 56 & 181 & 379 & 616 & 74 & 210 & 394 & 678 \\
Lies on the Serpent's Tongue & Kate Pearsall & Fantasy, Horror & 96,311 & Jan 7, 2025 & 24 & 73 & 192 & 377 & 642 & 84 & 209 & 377 & 670 \\
All the Water in the World & Eiren Caffall & Science Fiction & 98,082 & Jan 7, 2025 & 25 & 65 & 195 & 413 & 673 & 97 & 251 & 402 & 750 \\
Holmes is Missing & James Patterson & Mystery, Thriller & 98,497 & Jan 2, 2025 & 25 & 87 & 214 & 382 & 683 & 101 & 246 & 391 & 738 \\
The Lodge & Kayla Olson & Romance & 104,102 & Jan 7, 2025 & 26 & 81 & 205 & 375 & 661 & 98 & 231 & 380 & 709 \\
Switching Graves & Jen Stevens & Dark, Gothic & 107,565 & Jan 3, 2025 & 27 & 85 & 230 & 461 & 776 & 90 & 237 & 417 & 744 \\
So Not My Type & Dana Hawkins & Romance & 107,728 & Dec 12, 2024 & 27 & 66 & 186 & 375 & 627 & 75 & 220 & 384 & 679 \\
Close Your Eyes & Teresa Driscoll & Thriller & 107,933 & Jan 1, 2025 & 27 & 90 & 240 & 489 & 819 & 99 & 283 & 528 & 910 \\
Kingdom of Faewood & Krista Street & Fantasy & 108,780 & Jan 3, 2025 & 28 & 92 & 225 & 447 & 764 & 92 & 220 & 424 & 736 \\
Bitter Passage: An Allegheny Beckham Novel & Colin Mills & Mystery & 111,603 & Jun 22, 2024 & 28 & 72 & 220 & 456 & 748 & 95 & 241 & 460 & 796 \\
The Three Lives of Cate Kay & Kate Fagan & Fiction, Mystery & 113,253 & Jan 7, 2025 & 29 & 105 & 248 & 459 & 812 & 104 & 255 & 424 & 783 \\
Some Other Time & Angela Brown & Fiction & 114,761 & Jan 1, 2025 & 29 & 85 & 223 & 436 & 744 & 99 & 235 & 386 & 720 \\
\midrule
Average (Total) & - & - & 100,507 & - & 25 (407) & 76 (1209) & 203 (3252) & 403 (6445) & 682 (10916) & 87 (1382) & 226 (3616) & 401 (6409) & 714 (11417) \\
\bottomrule
\end{tabular}%
} 
\caption{Statistics and details of the novels used for constructing \algname{}. All novels' are purchased as an electronic copy. Due to copyright restrictions, we do not release the full text of the books. *Note that for each chunk, two key-fact trees and two queries are created corresponding to the two summarization perspectives (analytical and narrative).}
\label{tab:book_info}
\end{table*}

Our dataset comprises 16 books, which serve as the original data sources for this task. These books were purchased from Amazon. Due to copyright restrictions, we do not release the full text of the books; instead, we provide only the queries, summaries, key fact trees, and evaluation labels. Table~\ref{tab:book_info} presents detailed information about the selected books.

To process the text, we employ \texttt{tiktoken}\footnote{\url{https://github.com/openai/tiktoken}}, a tokenization library developed by OpenAI, to segment the text into tokens and compute token counts. Each book is divided into multiple chunks of approximately 4,000 tokens, ensuring that sentence boundaries remain intact during segmentation. Table~\ref{tab:book_info} summarizes the statistical properties of these chunks, including the number of validated key facts.

\section{Key-fact Hierarchy \& Query Type Details}

\begin{table*}[t!]
  \centering
  \scriptsize{}
  \renewcommand{\arraystretch}{0.8}
  \setlength{\tabcolsep}{3pt}
  \begin{tabular*}{\textwidth}{@{\extracolsep{\fill}}
     >{\centering\arraybackslash}m{0.12\textwidth}  % first column, vertically centered
     M{0.4\textwidth}                               % Analytical
     M{0.4\textwidth}                               % Narrative
  }
  \toprule
  & \multicolumn{1}{c}{Analytical}
    & \multicolumn{1}{c}{Narrative} \\
  \midrule
  Definition
    & Analytical perspective focuses on thematic elements, implications, character development, and symbolic patterns, examining how these literary components build toward deeper meaning and authorial intent.
    & Narrative perspective emphasizes chronological storytelling, key events, and plot developments, concentrating on how the storyline unfolds and progresses through the text. \\
  \midrule

  Root Definition 
  & A single concise sentence summarizing the overarching purpose, argument, or main analytical insight of the text.
  & A single concise sentence capturing the main idea or overarching sequence of events in the text.
  \\
  \midrule

  Branch Definition 
  & Key supporting ideas, arguments, or elements that develop the overarching purpose or insight, including significant stages, relationships, or turning points in the text. 
  & Key supporting events or developments that progress the narrative logically, including major stages, actions or transitions.
  \\
  \midrule

  Leaf Definition
  & Specific evidence, minor details, or examples that provide additional support or elaboration for each branch. 
  & Specific details, minor events, or pieces of evidence that provide additional clarity or elaboration for each branch. 
  \\
  \midrule
  Query Example
    & How do the social rejection and personal challenges Holmes faces at the bar, his subsequent return home with Callie Brett's assistance, and the professional and personal challenges faced by Poe and Holmes, including the discovery of twins, collectively illustrate the overarching themes of vulnerability, trust, and commitment in the narrative?
    & Provide a detailed summary of the events involving Holmes at the bar, his interaction with Callie Brett, the subsequent health incident, and the developments with Poe and Grey, including their medical appointment and the team's commitment to a crime-writers' convention? \\
  \bottomrule
  \end{tabular*}
  \caption{Definitions of two summarization perspectives and their example queries.}
  \label{tab:keyfact-query-definition}
\end{table*}


Table~\ref{tab:keyfact-query-definition} shows the detailed definitions of each level in our key-fact hierarchy and the corresponding queries across analytical and narrative perspectives. This taxonomy forms the foundation of our key-fact tree generation and query generation components, enabling the systematic construction of our benchmark across varying granularities of information abstraction and contrasting summarization perspectives.



\section{Model details}\label{appendix:model_details}

\begin{table}[h!]
\centering 
\renewcommand{\arraystretch}{1.1}
\setlength{\tabcolsep}{4pt}
\resizebox{\linewidth}{!}{%
\begin{tabular}{ccccc}
    \toprule
    Model Type & Model Name & \makecell{Context \\ Length} & \makecell{Knowledge \\ Cutoff} & \makecell{Hugging Face Checkpoints \\ \& Official API Version} \\ 
    \midrule
    \multirow{4}{*}{\makecell{Commercial \\Models}} 
        & GPT-4o & 128K & Oct, 2023 & gpt-4o-2024-08-06 \\
        & GPT-4o-mini & 128K & Oct, 2023 & gpt-4o-mini-2024-07-18\\
        & Claude-3-5-Sonnet & 200K & Apr, 2024 & claude-3-5-sonnet-20240620\\
        & Claude-3-5-Haiku & 200K & Jul, 2024 & claude-3-5-haiku-20241022\\
    \midrule
    \multirow{4}{*}{\makecell{Open-Source \\ Models}} 
        & LLaMA-3.1-405B & 128K & Dec, 2023 & meta-llama/Llama-3.1-405B-Instruct\\
        & LLaMA-3.1-8B & 128K & Dec, 2023 & meta-llama/Llama-3.1-8B-Instruct\\
        & Qwen2.5-32B-Instruct & 128K & - &  Qwen/Qwen2.5-32B-Instruct\\
        & DeepSeek-R1-Distill-Qwen-32B & 128K & - & deepseek-ai/DeepSeek-R1-Distill-Qwen-32B\\
    \bottomrule
\end{tabular}%
}
\caption{Overview of model specifications including their types, context window sizes, and knowledge cutoff dates. Note that GPT-4o-mini is also used as the baseline model for automated summary evaluation (Section ~\ref{tab:humaneval_summary_auto_evaluation}. \cmtLee{add model precision - see unisumeval 2 paper}}
\label{tab:model_overview}
\end{table}

We compare various commercial and open-source large language models, highlighting their context lengths and knowledge cutoffs. The details of these models are presented in Table~\ref{tab:model_overview}. For open-source LLMs, we use instruction-tuned versions. For commercial models, we use official APIs. We set the temperature parameter to \cmtLee{temp param} and the model precision is set to \cmtLee{precision e.g., 8bit}.



\section{Evaluation Details}\label{appendix:eval_details} 
Our work follows \cite{song2024finesure} to do the summarization evaluation. The evaluation consists two tasks: \textit{Fact verification} and \textit{Key-fact alignment}.
\subsection{Fact Verification}
To evaluate faithfulness, we conduct fact-checking using GPT-4o as the evaluator. Table~\ref{tab:fact_checking_eval} provides the fact-checking prompt.The summary is split into individual sentences, and the original text from which the query was generated is provided as context. The LLM labels each summary sentence as either faithful (1) or unfaithful (0). The LLM assigns a binary label to each sentence: faithful (1) or unfaithful (0). Additionally, following the taxonomy in Table~\ref{tab:error-categories}, each unfaithful sentence is categorized, with an accompanying explanation.
% The faithfulness score is then computed as: 
% \begin{equation}
% \text{Faithfulness} = \frac{\sum_{s \in S} \mathbb{1} (s = 1)}{|S|}
% \end{equation}

% where \( S \) is the set of summary sentences, and \( \mathbb{1}(s = 1) \) is an indicator function that equals 1 if the sentence is faithful and 0 otherwise.


\begin{table}[h!]
\begin{center}
\renewcommand{\arraystretch}{1.1}
\setlength{\tabcolsep}{3pt}
\footnotesize  % 使用更小的字体以适应单列
\begin{tabular}{p{0.20\columnwidth}p{0.25\columnwidth}p{0.55\columnwidth}}
    \toprule
    \textbf{Error Category} & \textbf{Error Type} & \textbf{Description} \\
    \midrule
    Extrinsic Error & Out-of-article error & The summary introduces facts, opinions, or information not found in or reasonably inferrable from the text  \\
    \midrule
    \multirow{3}{*}{Intrinsic Error} & Entity error & Incorrect reference to key subjects/objects (e.g., wrong names, numbers, pronouns) \\
    \cmidrule{2-3}
    & Relation error & Mistakes in semantic relationships (e.g., incorrect verbs, prepositions, adjectives)  \\
    \cmidrule{2-3}
    & Sentence error & Multiple errors causing the entire sentence to contradict the text \\
    % \midrule
    % No error & The summary statement aligns with the text's content \\
    \bottomrule
\end{tabular}
\end{center}
\caption{Summary Error Categories with Examples}
\label{tab:error-categories}
\end{table}




\begin{table}[h!]
\begin{center}
\renewcommand{\arraystretch}{1.1}
\setlength{\tabcolsep}{3pt}
\footnotesize  % 使用更小的字体以适应单列
\begin{tabular}{p{0.3\columnwidth}p{0.7\columnwidth}}
    \toprule
    \textbf{Error Type} & \textbf{Description} \\
    \midrule
    Out-of-article error & The summary introduces facts, opinions, or information not found in or reasonably inferrable from the text  \\
    \midrule
    Entity error & Incorrect reference to key subjects/objects (e.g., wrong names, numbers, pronouns) \\
    \midrule
    Relation error & Mistakes in semantic relationships (e.g., incorrect verbs, prepositions, adjectives)  \\
    \midrule
    Sentence error & Multiple errors causing the entire sentence to contradict the text \\
    % \midrule
    % No error & The summary statement aligns with the text's content \\
    \bottomrule
\end{tabular}
\end{center}
\caption{Summary Error Categories with Examples}
\label{tab:error-categories}
\end{table}

\subsection{Key-fact Alignment}
We use key-fact alignment to compute both completeness and conciseness scores. Table~\ref{tab:key_fact_alignment_eval} provides the key-fact alignment prompt. The summary sentences, the query, the key-fact tree generated from the original text, and the original text itself are provided to the evaluator (GPT-4o).  


%% This part is commented as we put the formulas now in the main body
% \paragraph{Completeness:} Each key fact in the key fact tree is labeled as contained (1) or not contained (0) in the summary. If a key fact is labeled as 1, the LLM also identifies the index of the summary sentence that contains it. The completeness score is calculated as:

% \begin{equation}
% \text{Completeness} = \frac{\sum_{k \in K} \mathbb{1} (k = 1)}{|K|}
% \end{equation}
% where \( K \) is the set of key facts, and \( \mathbb{1}(k = 1) \) indicates whether the key fact is present in the summary.

% \paragraph{Conciseness:} We calculate conciseness based on the number of summary sentences that contribute to covering key facts. The conciseness score is defined as:

% \begin{equation}
% \text{Conciseness} = \frac{\sum_{s \in S} \mathbb{1} (s \text{ mentions a key fact})}{|S|}
% \end{equation}
% where \( S \) is the set of summary sentences, and \( |S| \) represents the total number of summary sentences.  
% \( \mathbb{1}(s \text{ mentions a key fact}) \) is an indicator function that equals 1 if the summary sentence \( s \) contains at least one key fact, and 0 otherwise.

% This approach ensures a structured and fine-grained evaluation of faithfulness, completeness, and conciseness using LLM-based assessment.



\subsection{Mid-degradation Rate}

\tobefilled{}
\cmtLee{formally define the mid degradatuion rate formula}





\section{Evaluation Performance}\label{appendix:evaluation_performance}
\input{figures/appendix/data_table/table_for_figure3}
In the following section, we show the detailed table for the recall performance across different levels and different positions in Table~\ref{tab:recall_total}.

\cmtLee{need to change it}


\section{Annotator Recruitment Details}\label{apppendix:annotator_recruitment}
\tobefilled{}


\subsection{Expert Annotators}

Used for key-fact validation, query eavlaution and automated evaluiation validation




\subsection{Crowdsourced Annotators}


used for the automated evaluation baseline

% \begin{table*}[t]
% \centering
% \footnotesize
% \renewcommand{\arraystretch}{1.2}
% \setlength{\tabcolsep}{2pt}
% \resizebox{\textwidth}{!}{
% \begin{tabular}{l
% >{\centering\arraybackslash}p{1.2cm}
% >{\centering\arraybackslash}p{1.2cm}
% >{\centering\arraybackslash}p{1.2cm}
% >{\centering\arraybackslash}p{1.2cm}
% >{\centering\arraybackslash}p{1.2cm}
% >{\centering\arraybackslash}p{1.2cm}
% >{\centering\arraybackslash}p{1.2cm}
% >{\centering\arraybackslash}p{1.2cm}
% >{\centering\arraybackslash}p{1.2cm}
% >{\centering\arraybackslash}p{1.2cm}
% >{\centering\arraybackslash}p{1.2cm}
% >{\centering\arraybackslash}p{1.2cm}
% }
% \toprule
% Level &
% \multicolumn{2}{c}{GPT-4o} &
% \multicolumn{2}{c}{GPT-4o-Mini} &
% \multicolumn{2}{c}{LLaMA-3.1-405B} &
% \multicolumn{2}{c}{LLaMA-3.1-8B} &
% \multicolumn{2}{c}{Claude-3.5-Sonnet} &
% \multicolumn{2}{c}{Claude-3.5-Haiku} \\
% \cmidrule(lr){2-3} \cmidrule(lr){4-5} \cmidrule(lr){6-7} \cmidrule(lr){8-9} \cmidrule(lr){10-11} \cmidrule(lr){12-13}
% & Ana & Nar & Ana & Nar & Ana & Nar & Ana & Nar & Ana & Nar & Ana & Nar \\
% \midrule
% Root   & 1.1  & -5.4 & -3.0  & -11   & 3.3  & 0.04 & -0.00 & -3.0  & 7.9  & -4.8 & 6.9  & 3.4 \\
% Branch & 0.6  & 3.1  & 1.2   & 5.5   & 1.4  & 8.4  & 3.8   & -6.9  & 13   & 1.7  & 11   & 0.8 \\
% Leaf   & -8.1 & 2.6  & -8.9  & 6.6   & -16  & 9.3  & -1.6  & -9.8  & 2.9  & 1.9  & -9.3 & 0.3 \\
% Total  & -4.7 & 0.7  & -8.0  & 3.7   & -9.5 & 4.8  & 1.5   & -9.0  & 8.3  & -2.6 & -0.9 & -0.9 \\
% \bottomrule
% \end{tabular}
% }
% \caption{Pearson correlation coefficients ($r$) between summary length and recall across levels and models. Each value is scaled by $10^{-2}$.}
% \label{tab:pearson_corr}
% \end{table*}


\section{Supplementary Analysis}\label{appendix:supplement}

In this Appendix, we provide supplementary analysis that provide further insights into our primary findings. 


\subsubsection{Faithfulness error distribution.}\label{appendix:faithfulness_error_analysis}
\begin{table}[h]
\centering
\resizebox{\columnwidth}{!}{%
\begin{tabular}{@{}lc@{}}
\toprule
\textbf{Category}                                                                    & \textbf{\% of Total Faithfulness Errors} \\ \midrule
(A) Extrinsic Error                                                                  & 5\%                                      \\
(B) Intrinsic Error                                                                  & 95\%                                     \\ \midrule
\textbf{\begin{tabular}[c]{@{}l@{}}Subcategories of \\ Intrinsic Error\end{tabular}} & \textbf{\% of (B) Intrinsic Error}       \\ \midrule
Entity Error                                                                         & 45\%                                     \\
Relation Error                                                                       & 54\%                                     \\
Sentence Error                                                                       & 1\%                                      \\ \bottomrule
\end{tabular}%
}
\caption{Faithfulness error type distribution. The result is averaged over the six summarizers, excluding the two Qwen-2.5-32B models (Instruct and R1-distill).}
\label{tab:error_type}
\end{table}











\input{figures/appendix/prompt/keyfact_tree_generation/analytical}
\input{figures/appendix/prompt/keyfact_tree_generation/narrative}
\input{figures/appendix/prompt/keyfact_tree_validation/faithfulness}
\input{figures/appendix/prompt/keyfact_tree_validation/subjectivity}
\input{figures/appendix/prompt/keyfact_tree_validation/significance}
\input{figures/appendix/prompt/queries_generation/analytical_queries}
\input{figures/appendix/prompt/queries_generation/narrative_queries}
\input{figures/appendix/prompt/summaries_evaluation/fact_checking}
\input{figures/appendix/prompt/summaries_evaluation/keyfact_alignment}
